# Supplementary material for: 3QFP: Efficient neural implicit surface reconstruction using Tri-Quadtrees and Fourier feature Positional encoding
Source: arXiv:2401.07164 source file (2024-04-07)
Supplement: Supplementary file 1 [file supplementary.tex]

Assuming the generated predicted mesh and the ground-truth mesh are $\mathcal{M}_{\text{pred}}$ and $\mathcal{M_{\text{gt}}}$ respectively.
The evaluation metrics are defined as follows:

\textbf{Accuracy} (lower better $\downarrow$): Mean Absolute Distance (\textit{MAD}) of points sampled from the predicted mesh $\mathcal{M_{\text{pred}}}$ to the closest surface on the ground truth mesh $\mathcal{M}_{\text{gt}}$.

\textbf{Completeness} (lower better $\downarrow$): \textit{MAD} of points sampled form the ground truth mesh $\mathcal{M}_{\text{gt}}$ to the closest surface on the predicted mesh $\mathcal{M_{\text{pred}}}$.

\textbf{Recall} (higher better $\uparrow$): The percentage of points sampled from the ground truth mesh that have closest absolute distance to the predicted mesh within a threshold $\tau_{r}$.

\textbf{IoU} (higher better $\uparrow$): \textit{IoU} is defined as the volumetric intersection of the $\mathcal{M}_{\text{pred}}$ and $\mathcal{M}_{\text{gt}}$ over the union. $\text{IoU} \doteq \frac{|\mathcal{M}_{\text{pred}} \cap \mathcal{M}_{\text{pred}}|}{|\mathcal{M}_{\text{pred}} \cup \mathcal{M}_{\text{pred}}|}$.

Considering the requirements in the real applications, we also need to take the resources usage and running time into account.
Specifically, we should consider the following evaluation matrices.

\textbf{GPU-usage} (lower better $\downarrow$): The GPU memory usage to process one frame (or given certain number of points).

\textbf{Running-time} (lower better $\uparrow$): the time usage when processing an input frame.
